# Supplementary material for: On Non-Random Missing Labels in Semi-Supervised Learning
Source: arXiv:2206.14923 source file (2022-06-29)
Supplement: Supplementary file 1 [file appendix.tex]

\section{Appendix}

\subsection{Implementation Details}
As mentioned in Section 5.1, we used almost identical hyper-parameters as FixMatch~\citep{fixmatch} on CIFAR-10, CIFAR-100, STL-10 and mini-ImageNet. Here, we provide a complete list of hyper-parameters in Table~\ref{tab:param}, where  xx/xx denote the parameters in FixMatch/Ours and xx is the common parameter.

\begin{table*}[ht]
\centering

\setlength{\tabcolsep}{1.2mm}{

\begin{tabular}{|l| p{1cm}<{\centering}|c|l|l|l|}
\hline
 & \multicolumn{1}{l|}{Notation} &  \multicolumn{1}{l|}{\makecell[c]{CIFAR-10\\iNaturalist-20}} & \makecell[c]{CIFAR-100\\iNaturalist-50} & STL-10 & mini-ImageNet \\ \hline
confidence threshold & $\tau_o$ & \multicolumn{4}{c|}{0.95} \\
unlabel loss weight & $\lambda_u$ & \multicolumn{4}{c|}{1} \\
\#unlabeled/\#label in batch & $\eta$ & \multicolumn{4}{c|}{7} \\
labeled data batch-size & $b$ & \multicolumn{4}{c|}{64} \\
start learning rate & $lr$ & \multicolumn{4}{c|}{0.03} \\
momentum & $m$ & \multicolumn{4}{c|}{0.9} \\
CAP coefficient & $\mu$ & \multicolumn{4}{c|}{NA/0.99} \\
CAI coefficient & $\beta$ & \multicolumn{4}{c|}{NA/0.5} \\ \hline
weight decay & $w$ & 0.0005 & \multicolumn{1}{c|}{0.001/0.0015} & \multicolumn{1}{c|}{0.0005} & \multicolumn{1}{c|}{0.0005} \\ \hline
\end{tabular}}

\caption{Complete list of hyper-parameters for CIFAR-10, CIFAR-100, STL-10 and mini-ImageNet.}
\label{tab:param}
\end{table*}

For DARP~\citep{DARP}, the original implementation needs abundant labeled data as the validation set to estimate the unlabeled data distribution, which is not practical in our case (the minimal number of labeled data of classes is 1). 
As an alternative, we provide DARP with the ground truth unlabeled data distribution.

\subsection{Double Robustness of the DR estimator}
\textbf{Scenario 1}: CAP is correct, \ie, the propensity $p^{(i)}$ successfully reflects the data missing mechanism. We have:
\begin{align}
\mathcal{L}_\text{CAI}+\mathcal{L}_\text{supp} = \frac{1}{N} \sum\limits_{i=1,\cdots,N}{(1-\frac{1-m^{(i)}}{p_i}) \mathcal{L}_u(x^{(i)},q^{(i)}) \  \mathbb{I}(\text{con}(q^{(i)})>\tau) }.
\end{align}
The expectation of it over $M$ is written as:
\begin{align}
E_M[\mathcal{L}_\text{CAI}+\mathcal{L}_\text{supp}] & = E_M[\sum\limits_{i=1,\cdots,N}{(1-\frac{1-m^{(i)}}{p^{(i)}}) \mathcal{L}_u(x^{(i)},q^{(i)}) \  \mathbb{I}(\text{con}(q^{(i)})>\tau) }] \\
& = \sum\limits_{i=1,\cdots,N}{E_{m^{(i)}}[(1-\frac{1-m^{(i)}}{p^{(i)}}) \mathcal{L}_u(x^{(i)},q^{(i)}) \  \mathbb{I}(\text{con}(q^{(i)})>\tau) ]}. \label{eq:proof1}
\end{align}
As $E_{m^{(i)}}[1-m^{(i)}] = p^{(i)}$ is the probability that a data is labeled, we have Eq.~\ref{eq:proof1} equals 0.
\\

\textbf{Scenario 2}: CAI is correct, \ie, the imputed label plays the same role as the true label:
\begin{small}
\begin{align}
\mathcal{L}_\text{CAP}+\mathcal{L}_\text{supp} &= \frac{1}{N} \sum \limits_{i=1,\cdots,N}{\frac{(1-m^{(i)})\mathcal{L}_s(x^{(i)},y^{(i)})}{p^{(i)}}} -\frac{1}{N} \sum \limits_{i=1,\cdots,N}{(1-m^{(i)}) \mathcal{L}_s(x^{(i)},y^{(i)})} \\ \nonumber
& + \frac{1}{N} \sum \limits_{i=1,\cdots,N}{(1-m^{(i)}-\frac{1-m^{(i)}}{p^{(i)}}) \mathcal{L}_u(x^{(i)},q^{(i)}) \  \mathbb{I}(\text{con}(q^{(i)})>\tau) }\\ \nonumber
& = \frac{1}{N} \sum \limits_{i=1,\cdots,N}{(\frac{1-m^{(i)}}{p^{(i)}}-(1-m^{(i)})\mathcal{L}_s(x^{(i)},y^{(i)}))} \\ \nonumber
& -  \frac{1}{N} \sum\limits_{i=1,\cdots,N}{(\frac{1-m^{(i)}}{p^{(i)}}-(1-m^{(i)})\mathcal{L}_u(x^{(i)},q^{(i)}) \  \mathbb{I}(\text{con}(q^{(i)})>\tau))} \\ \nonumber
&= \sum\limits_{i=1,\cdots,N}{(\frac{1-m^{(i)}}{p^{(i)}}-(1-m^{(i)})) (\mathcal{L}_s(x^{(i)},y^{(i)}) - \mathcal{L}_u(x^{(i)},q^{(i)}) \  \mathbb{I}(\text{con}(q^{(i)})>\tau) )   },
\end{align}
\end{small}
whose expectation equals to 0 as the second term in summation is expected to be 0 when imputation is ideal.

\subsection{Algorithm}

\begin{algorithm}
\setstretch{1.3}
\caption{ Our Class-Aware Doubly Robust Method}
\begin{algorithmic}[1] %每行显示行号
    \settowidth{\maxwidth}{$mmmm$}% use the widest one
    \State \algalign{\textbf{Input}}{:}\  $ D_L$,   $ D_U$   
    \Comment{labeled and unlabeled data}
    \State \algalign{\textbf{Input}}{:}  model $\theta_0$ , strong augmentation $\mathcal{A}$, threshold $\tau_o$
    \State \algalign{\textbf{Output}}{:}\  $\theta$
    \State  Initialize $\theta_0$ randomly, Iteration $i=0$, $P(Y)$ is uniform
    \For{$i < \text{MaxIter}$ } 
    \State $\{X_L,Y_L\} \leftarrow D_L$, $\{X_U\} \leftarrow D_U$
    \Comment{sample a mini-batch}
    \State $\text{Output}_L(\theta)\cup \text{Output}_U(\theta) \gets f_\theta(\{X_L,Y_L\} \cup \{X_U\})$ 
    \Comment{Model prediction}
    \State $P(Y|X ; \theta) \gets \Call{Softmax}{\text{Output}_L(\theta)\cup \text{Output}_U(\theta)}$
    \Comment{softmax probability}
    
    \State \textit{\# For supervised labeled data:}
    \State $P(Y), P(Y;\theta) \gets \Call{CAP}{\text{Output}_L(\theta)\cup \text{Output}_U(\theta), P(Y)}$ 
    \Comment{ CAP }
    
    \State $\mathcal{L}_s(X_L,Y_L) \gets \Call{CAP-Loss}{P(Y_L|X_L;\theta), P(Y;\theta)}$
    \Comment{ Eq. (5-9) }
    
    \State \textit{\# For imputed unlabeled data:}
    \State $Q, \text{con(Q)} \gets \Call{Max}{\text{Output}_U(\theta)}$ 
    \Comment{imputed label with confidence}
    \State $\tau \gets \tau_o, P(Y), Q $ 
    \Comment{ Eq. (11)}
    \State $\mathcal{L}_u(X_U) \gets \Call{CAI-Loss}{\text{Output}_U(\theta), \tau}$
    \Comment{ Eq. (13)}
    \State \textit{\# Model update:}
    \State $\theta \gets \theta - \nabla_{\theta}\Call{DR-Loss}{\mathcal{L}_s(X_L,Y_L) , \mathcal{L}_u(X_U), X_L, P(Y;\theta), \tau }$
    \Comment{ Eq. (14)}
    % \State $\text{Output}_l \  \gets \Call{InverseWeight}{\text{Output}_l,{p}_u} $ 
    % \Comment{ \eqref{equ:ourMLE}}
    
    \EndFor 
    \State \algalign{\textbf{Return}}{\theta}
\end{algorithmic}
\label{alg:DR}
\end{algorithm}

\subsection{More Experiments}

\subsubsection{More Comparisons of Labeling Dependence on Classes}
In this section, we performed experiments with the dependence of labeling on class varying in the intermediate range by increasing the labeling imbalance ration $\gamma$ from 1 to 200 gradually. As shown in Table~\ref{tab:ab_gamma}, our method can consistently boost the performance of baseline FixMatch under different levels of label dependence. Besides, the improvement is more significant with larger $\gamma$, \ie, the high dependence of labeling on class. This observation is reasonable since the baseline method gradually fails to handle the data distribution shift between the labeled and unlabeled data in challenging MNAR problems.

\begin{table*}[ht]
\vspace{-0.05in}
\centering

\setlength{\tabcolsep}{1.98mm}{
  
\begin{tabular}{lllcccccccc}
\toprule
\hline
\multicolumn{2}{l}{\textbf{Methods}}     &   & $\gamma$ = 1 & 2           & 5             & 10            & 20          & 50          & 100         & 200         \\ \cline{1-2} \cline{4-11}
\multicolumn{2}{l}{FixMatch} & & 78.54   & 76.77 & 74.71   & 70.53& 66.79 & 59.13 & 54.78 & 50.62  \\
\multicolumn{2}{l}{Ours}  &   & 79.02   & 77.71 & 76.32 & 74.37 & 73.47 & 70.06 & 64.47 & 63.30\\ \hline
\bottomrule
\end{tabular}}
\vspace{-0.05in}
\caption{Comparison of mean accuracies (\%) under different labeling dependence on the class. We alter the imbalance ratio $\gamma$ of the labeled data in the intermediate range from 1 to 200, where $\gamma=1$ is the case where the label is missing completely at random. The experiments are conducted on CIFAR-100, and we keep $N_{max}=200$ across all settings.}
\label{tab:ab_gamma}
\vspace{-0.05in}
\end{table*}

\subsubsection{Application to iNaturalist}
To apply our methods to real-data MNAR occasions, we conducted experiments on the subsets of iNaturalist~\citep{iNature}, a real-world dataset comprised of the natural images and labels collected from a citizen science website\footnote{\url{www.inaturalist.org}}. iNaturalist has two popular versions, iNaturalist-2018 for long-tailed recognition\footnote{\url{https://sites.google.com/view/fgvc5/competitions/inaturalist}} and iNaturalist-2021 for nearly balanced data recognition\footnote{\url{https://sites.google.com/view/fgvc8/competitions/inatchallenge2021}}. As iNaturalist-2021 supplements iNaturalist-2018 with abundant additional data in their overlapped classes, these two versions can be naturally used for our MNAR setting in SSL. Specifically, we sampled $N$ classes from the iNaturalist dataset, where the data in iNaturalist-2018 are used as the labeled data and the additionally released data in iNaturalist-2021 as the unlabeled. Figure~\ref{fig:iNature} depicts the details of our 20-class subset, and the data distribution of 20/50-class subsets are shown in Figure~\ref{fig:iNature}(b) and Figure~\ref{fig:iNature50} separately, where an obvious imbalanced distribution over the labeled data is observed.

\begin{figure}[t]
\centering
\includegraphics[width=0.9\linewidth]{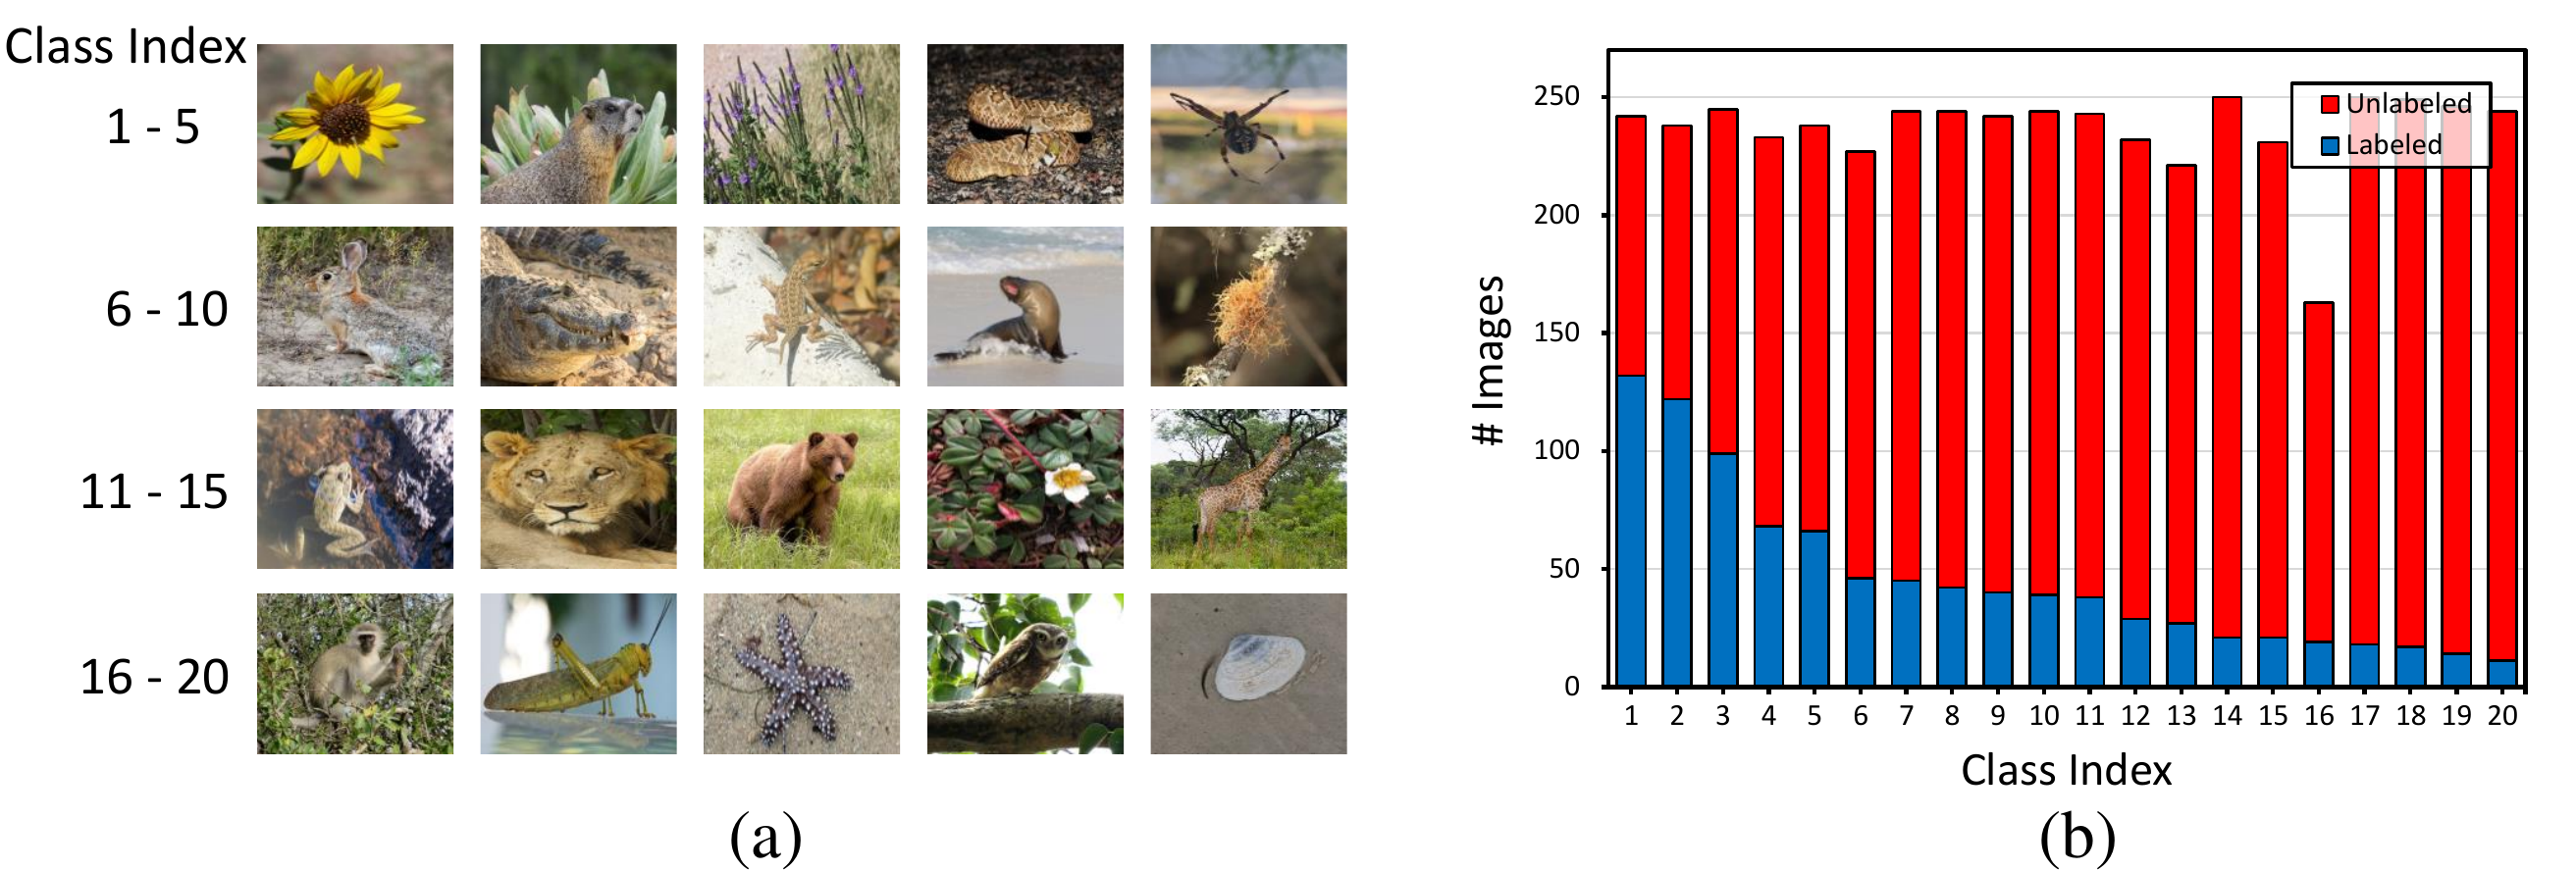}
\vspace{-0.05in}
\caption{Details about our constructed 20 classes subset of the iNaturalist dataset. (a) The example image for each class. (b) Class distribution of the labeled and unlabeled training data.}
\label{fig:iNature}
\end{figure} 

\begin{figure}[t]
\centering
\includegraphics[width=0.9\linewidth]{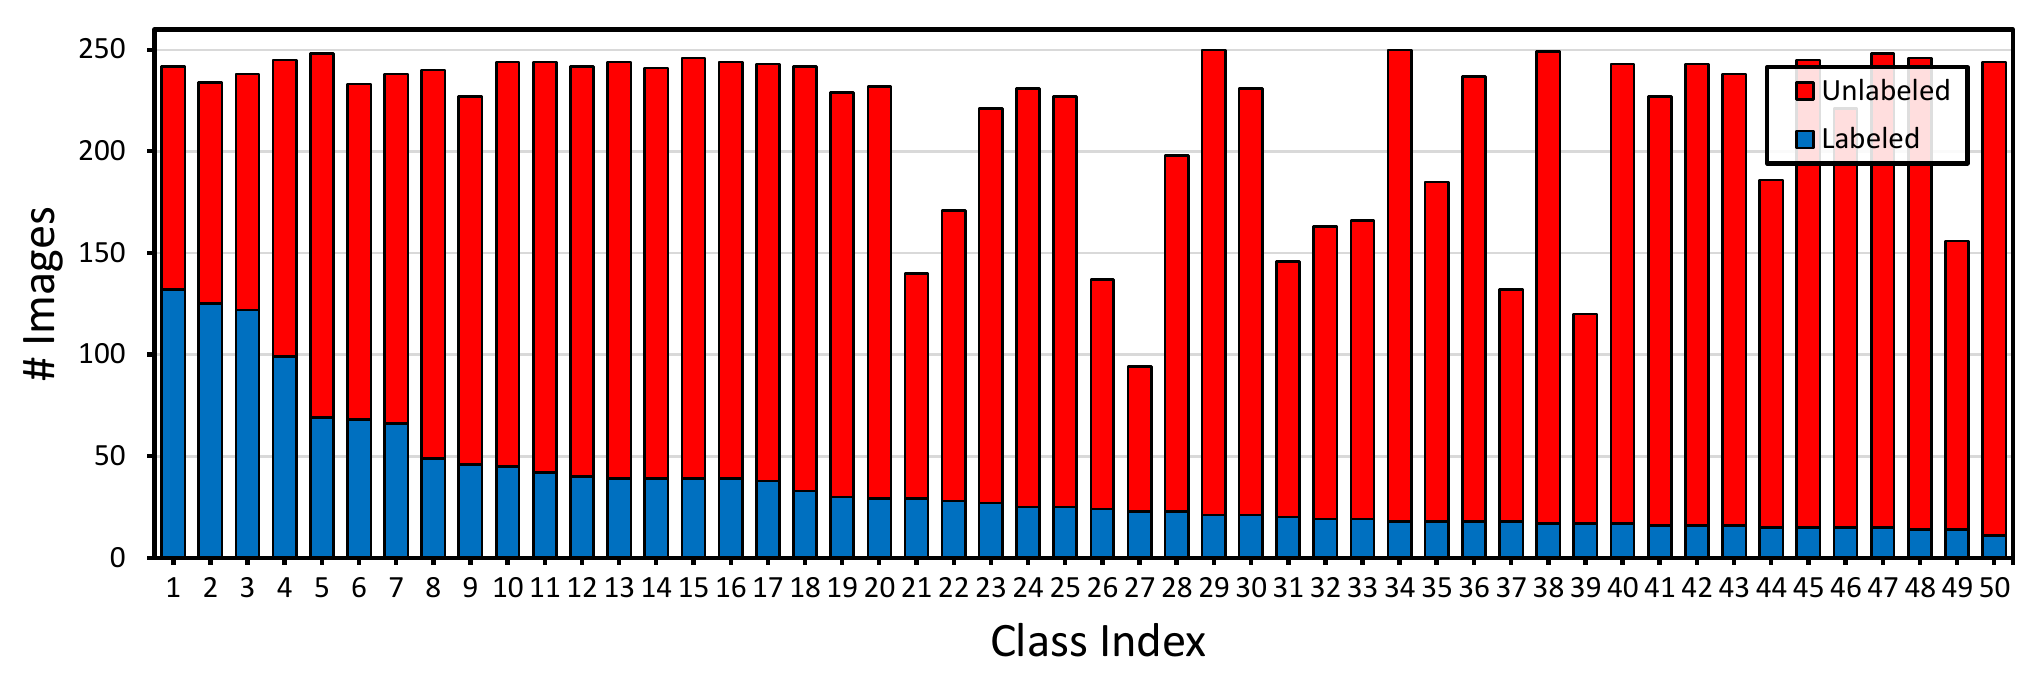}
\vspace{-0.05in}
\caption{Class distribution of the labeled and unlabeled training data in our constructed 50 classes subset of the iNaturalist dataset.}
\label{fig:iNature50}
\end{figure}

\begin{table*}[ht]
\centering
\vspace{-0.05in}

\setlength{\tabcolsep}{2.98mm}{
\begin{tabular}{llcc}
\toprule
\hline
           & \multicolumn{2}{c}{$N=20$}        & $50$ \\ \hline
Supervised & \multicolumn{2}{c}{25.30} &    17.09 \\ \hline
FixMatch        & \multicolumn{2}{c}{43.20} &  47.24    \\\hline
w/ \, CAP        & \multicolumn{2}{c}{48.80} &   \textbf{51.32}   \\
w/ \,  CAI        & \multicolumn{2}{c}{47.50} &    48.43  \\
w/o CADR   & \multicolumn{2}{c}{\underline{50.80}} &     49.48 \\
w/ \,  CADR & \multicolumn{2}{c}{\textbf{51.60}} &    \underline{50.14} \\ 
\hline
\bottomrule
\end{tabular}
}
\vspace{-0.05in}
\caption{Comparisons of mean accuracies (\%) on the iNaturalist-subsets between the fully-supervised method, FixMatch, and ours. We marked the \textbf{best} and \underline{second-best} accuracies.}
\label{tab:iNature}
\vspace{-0.05in}
\end{table*}

To train the dataset, we resize the images to $64\times64$, remove the overlapped images and sample 50 images per class from iNaturalist2021 for performance evaluation, and train each network with Wide ResNet (WRN)-28-2 by $2^{15}$ iterations. Other hyper-parameters are shown in Table~\ref{tab:param}. The performance comparisons are shown in Table~\ref{tab:iNature}. It shows that our proposed methods outperform the baseline FixMatch by large margins, demonstrating the effectiveness of our methods in handling real-world imbalanced labeled data.

\subsubsection{More Ablation on Other Baselines}
In this section, we perform the ablation experiments on more baseline methods, MixMatch~\citep{mixmatch} and RemixMatch~\citep{remixmatch}. As they do not have a threshold in label imputation, CAI is not directly applicable, and we only apply CAP on them.  As shown in Table~\ref{tab:ab_mix}, our method consistently boosts the performance, especially outperforming the baselines by large margins on CIFAR-10 and STL-10.

\begin{table*}[ht]
\vspace{-0.05in}
\centering

\setlength{\tabcolsep}{1.98mm}{
  
\begin{tabular}{lcccccccccc}
\toprule
\hline
           & \multicolumn{3}{c}{CIFAR-10} &  & \multicolumn{2}{c}{CIFAR-100} &  & STL-10 &  & mini-ImageNet \\ \cline{2-4} \cline{6-7} \cline{9-9} \cline{11-11} 
\textbf{Methods} & \textit{$\gamma$=20} & \textit{50} & \textit{100} & \textit{} & \textit{100} & \textit{200} & \textit{} & \textit{100} & \textit{} & \textit{100} \\ \hline
MixMatch   & 26.63    & 31.28   & 28.02   &      & 41.32    & 42.92   &  & 28.31  &  & 18.30         \\
w/ CAP     & 40.34    & 43.51   & 45.47   &      & 42.45    &  46.54   &  & 34.76  &  &  22.09             \\ \hline
ReMixMatch & 41.84    & 38.44   & 38.20   &      & 39.71    & 39.22   &  & 39.55  &  & 23.50         \\
w/ CAP     & 51.90    & 55.03   & 53.44   &      & 40.15    & 39.40   &  & 42.53  &  &  23.74            \\ \hline
\bottomrule
\end{tabular}}
\vspace{-0.05in}
\caption{Comparison of mean accuracies (\%) with more baselines. 
We alter the imbalance ratio $\gamma$ of labeled data and leave the unlabeled data balanced ($\gamma_u=1$). We keep $N_{max}=\gamma$ so that the least number of labeled data among all the classes is always 1.}
\label{tab:ab_mix}
\vspace{-0.05in}
\end{table*}

% \begin{table*}[ht]
% \vspace{-0.05in}
% \centering
% \renewcommand\arraystretch{1.1}
% \setlength{\tabcolsep}{1.98mm}{
  
% \begin{tabular}{llccc}
% \toprule
% \hline
%   \textbf{Methods}         &  & $\gamma=$ 20     & 50       &  100     \\ \cline{1-1} \cline{3-5} 
% MixMatch   &  & 26.63 / \ \ 2.18  & 31.28 / \ \  2.53  & 28.02 / \ \  1.75  \\
% + CAP       &  & 33.09 / 10.52 & 37.46 / 11.76 & 41.05 / 11.68 \\ \hline
% ReMixMatch &  & 41.84 / 24.25 & 38.44 / 22.07 & 38.20 / 12.62 \\
% + CAP       &  & 51.94 / 26.49 & 55.12 / 29.37 & 47.47 / 13.77 \\ \hline
% \bottomrule
% \end{tabular}}
% \vspace{-0.05in}
% \caption{Comparison of mean accuracies (\%) / geometric mean accuracies (GM Accu) (\%) with more baselines on CIFAR-10. 
% We alter the imbalance ratio $\gamma$ of labeled data and leave the unlabeled data balanced ($\gamma_u=1$). We keep $N_{max}=\gamma$ so that the least number of labeled data among all the classes is always 1.  }
% \label{tab:ab_mix}
% \vspace{-0.05in}
% \end{table*}
